# Supplementary material for: Conditional Contrastive Learning with Kernel
Source: arXiv:2202.05458 source file (2022-03-15)
Supplement: Supplementary file 1 [file submission_supple.tex]

% \documentclass{article} % For LaTeX2e
% \usepackage{iclr2022_conference,times}

% % Optional math commands from https://github.com/goodfeli/dlbook_notation.
% \input{math_commands.tex}


% \usepackage{float}

% \usepackage{wrapfig}

% % to compile a preprint version, e.g., for submission to arXiv, add add the
% % [preprint] option:
% %     \usepackage[preprint]{neurips_2021}

% % to compile a camera-ready version, add the [final] option, e.g.:
% %     \usepackage[final]{neurips_2021}

% % to avoid loading the natbib package, add option nonatbib:
% %    \usepackage[nonatbib]{neurips_2021}

% \usepackage[utf8]{inputenc} % allow utf-8 input
% \usepackage[T1]{fontenc}    % use 8-bit T1 fonts
% \usepackage{hyperref}       % hyperlinks
% \usepackage{url}            % simple URL typesetting
% \usepackage{booktabs}       % professional-quality tables
% \usepackage{amsfonts}       % blackboard math symbols
% \usepackage{nicefrac}       % compact symbols for 1/2, etc.
% \usepackage{microtype}      % microtypography
% \usepackage{graphicx}
% \usepackage{subcaption}
% \usepackage{xcolor}         % colors

% \hypersetup{
%     colorlinks = true,
%     linkbordercolor = {white},
%     citecolor={olive}
% }

% \usepackage{amsmath}
% \usepackage{amsthm}
% \usepackage{amssymb}
% \usepackage{multirow}
% \usepackage[ruled,vlined]{algorithm2e}
% \newtheorem{theorem}{Theorem}[section]
% \newtheorem{proposition}[theorem]{Proposition}
% \newtheorem{lemma}[theorem]{Lemma}

% \title{Appendix for Conditional Contrastive Learning with Kernel}
% % Authors must not appear in the submitted version. They should be hidden
% % as long as the \iclrfinalcopy macro remains commented out below.
% % Non-anonymous submissions will be rejected without review.

% \author{Antiquus S.~Hippocampus, Natalia Cerebro \& Amelie P. Amygdale \thanks{ Use footnote for providing further information
% about author (webpage, alternative address)---\emph{not} for acknowledging
% funding agencies.  Funding acknowledgements go at the end of the paper.} \\
% Department of Computer Science\\
% Cranberry-Lemon University\\
% Pittsburgh, PA 15213, USA \\
% \texttt{\{hippo,brain,jen\}@cs.cranberry-lemon.edu} \\
% \And
% Ji Q. Ren \& Yevgeny LeNet \\
% Department of Computational Neuroscience \\
% University of the Witwatersrand \\
% Joburg, South Africa \\
% \texttt{\{robot,net\}@wits.ac.za} \\
% \AND
% Coauthor \\
% Affiliation \\
% Address \\
% \texttt{email}
% }

% % The \author macro works with any number of authors. There are two commands
% % used to separate the names and addresses of multiple authors: \And and \AND.
% %
% % Using \And between authors leaves it to \LaTeX{} to determine where to break
% % the lines. Using \AND forces a linebreak at that point. So, if \LaTeX{}
% % puts 3 of 4 authors names on the first line, and the last on the second
% % line, try using \AND instead of \And before the third author name.

% \newcommand{\fix}{\marginpar{FIX}}
% \newcommand{\new}{\marginpar{NEW}}

% %\iclrfinalcopy % Uncomment for camera-ready version, but NOT for submission.
% \begin{document}


% \maketitle
% \appendix

% \input{sec/appendix}

% \newpage


% \bibliography{ref}
% \bibliographystyle{iclr2022_conference}

% \end{document}
